# Supplementary material for: PLAYER*: Enhancing LLM-based Multi-Agent Communication and Interaction in Murder Mystery Games
Source: arXiv:2404.17662 source file (2025-05-20)
Supplement: Supplementary file 1 [file removed-appendix.tex]

\section{The WellPlay Dataset} \label{WellPlay}

In this work, we leverage the \textit{Conan} dataset, originally constructed by \citet{conan-zhao2024}, which comprises scripts from MMGs, including detailed annotations of character relationships. %Our bilingual dataset, encompassing both Chinese and English versions, is derived from this foundational work. 
Our dataset consists of two main components: Scripts and Evaluation questions.
In this work, we utilise the \textit{Conan} dataset, originally constructed by \citet{conan-zhao2024}, which consists of bilingual scripts from MMGs in both Chinese and English. However, the original dataset only provides annotations for character relationships, which is insufficient for evaluating an agent’s understanding of the game, its ability to comprehend the current situation, and its capacity to make correct and reasonable decisions. To address this limitation, we designed a comprehensive set of evaluation questions and annotated the dataset accordingly. These questions are categorised into three distinct types, with corresponding examples presented in Table~\ref{tab:question_example}.

\subsection{Scripts}
Each script features distinct narratives for individual characters. We have rephrased the original script from the \textit{Conan} dataset into two parts:

\begin{enumerate}
    \item \textbf{Background Script}. For each character, there is a corresponding background script includes all the information from their perspective. For example, for \emph{``Sylvia Costa''} in the script \emph{``Death Wears White''}, it is: \\ \\
    \emph{You are the head nurse of the emergency ward.You climbed to this position for your hard work and were proud. You are a very professional person and highly appreciated by colleagues. This job is perfect for you, except for a problem - you have not made enough money. Your salary is actually not enough for you to live a decent life, far from paying enough to take care of Mother's overhead ...} \\
    \item \textbf{Personal Objectives}. For each character, there are corresponding objectives that guide their actions. For example, for \emph{``Sylvia Costa''} in the script \emph{``Death Wears White''}, it is: \\ \\
    \emph{1. Ensure that no one will discover your illegal organ trafficking activities; \\ 2. Ensure that the kidnappers leave without being injured or killing anyone - you want to ensure that the police do not investigate deeply enough to discover your organ trafficking. The further away you are from the police, the safer you feel; \\
    3. ...}
\end{enumerate}

\begin{table*}[h!]
\centering
\resizebox{ \linewidth}{!}{
\begin{tabular}{|c|c|l|}
\hline
\textbf{Type}      & \textbf{Aspects}      & \multicolumn{1}{c|}{\textbf{Examples (The correct answer has been highlighted in bold.)}}    \\ \hline
\begin{tabular}[c]{@{}c@{}}A\\ (score 10)\end{tabular}                 & Who  & \begin{tabular}[c]{@{}l@{}}Who killed Hans Li Morette?\\ 
\textbf{A. Gale Li Morette} \\
B.Nurse head {[}Sylvia Costa{]} \\ 
C. Drake Li Morette \\
D. Frank Bijeli\end{tabular}  \\ \hline
\multirow{26}{*}{\begin{tabular}[c]{@{}c@{}}B\\ (score 5)\end{tabular}} & How  & \begin{tabular}[c]{@{}l@{}}How did Hans Li Morette die?\\ \textbf{A. Shot to death} \\ B. Beaten to death \\ C. Poisoned to death by poison \\ D.Drowned by water\end{tabular}                                        \\ \cline{2-3} 
& Why  & \begin{tabular}[c]{@{}l@{}}What was the motive behind the killer killing Hans Li Morette?\\ 
A. Love killing \\
B. Vendetta \\
\textbf{C. Interest} \\
D. Accidental killing\end{tabular}                                       \\ \cline{2-3} 
& Relationship       & \begin{tabular}[c]{@{}l@{}}What is the relationship between Murderer and Victim Hans Li Morette?\\ 
A. Enemies \\
B. Colleague \\
C. Friend \\
\textbf{D. Wife}\end{tabular}          \\ \cline{2-3} 
& Where   & \begin{tabular}[c]{@{}l@{}}Where was Hans Li Morette killed?\\ 
A. Emergency room \\
B. Johnson’s House \\
\textbf{C. Laboratory} \\
D. Dressing room\end{tabular}  \\ \cline{2-3} 
& When  & \begin{tabular}[c]{@{}l@{}}When was Hans Li Morette killed?\\ A. This afternoon from 5:00 to 5:30 \\
\textbf{B. This afternoon from 6:30 to 7:00}\\ 
C. Tonight from 7:00 to 7:30 \\
D. This morning from 6:30 to 7:00\end{tabular}                            \\ \cline{2-3} 
   & Suspect    & \begin{tabular}[c]{@{}l@{}}Please select the two people you most suspect of killing Hans Li Morette\\ 
\textbf{A. Gale Li Morette} \\
B. Nurse head {[}Sylvia Costa{]} \\
C. Drake Li Morette \\
D. Frank Bijeli\end{tabular}    \\ \hline
\multirow{11}{*}{\begin{tabular}[c]{@{}c@{}}C\\ (score 2)\end{tabular}} & \begin{tabular}[c]{@{}c@{}}Three\\ relationships\end{tabular} & \begin{tabular}[c]{@{}l@{}}
What is the non-existent relationship between Hans Li Morette and Andrew Paloski?\\ 
A. Andrew Paloski is colleague of Hans Li Morette,\\ 
B. Andrew Paloski is mentor of Hans Li Morette,\\ 
C. Andrew Paloski is jealous of Hans Li Morette,\\ 
\textbf{D. Hans Li Morette is future daughter in law of Andrew Paloski}\end{tabular} \\ \cline{2-3} 
& \begin{tabular}[c]{@{}c@{}}Two\\ relationships\end{tabular}   & \begin{tabular}[c]{@{}l@{}}
What is the relationship between Father Tom and Tony?\\ 
\textbf{A. Tony is manipulated by x and deceived by x of Father Tom}\\ 
B. Father Tom is authority over x and student of Tony\\ 
C. Father Tom is student and ex-girlfriend of Tony\\ 
D. Father Tom is ex-girlfriend and admired by x of Tony\end{tabular}                      \\ \cline{2-3} 
& \begin{tabular}[c]{@{}c@{}}One\\ relationships\end{tabular}   & \begin{tabular}[c]{@{}l@{}}What is the relationship between Father Tom and Drake Li Morette?\\ 
\textbf{A. Drake Li Morette is doctor of Father Tom}\\ 
B. Father Tom is helped by Drake Li Morette\\ 
C. Father Tom is step-brother of Drake Li Morette\\ 
D. Father Tom is hate of Drake Li Morette\end{tabular}        \\ \hline
\end{tabular}}
\caption{Examples of Each Type of Our Evaluation Questions}
\label{tab:question_example}
\end{table*}

\section{MMGs Rules and Procedure} \label{appendix: Rules and Procedure}
\subsection{Detailed Rules}\label{appendix:Rules}

\paragraph{Rule 1:} The total number of players participating in the game depends on the script. There may be one or more players who are the murderer(s), while the rest are civilians.
\paragraph{Rule 2:} The goal of the game is for civilian players to collaborate and face a meticulously planned murder case together, collecting evidence and reasoning to identify the real murderer among the suspects, all the while ensuring they are not mistaken for the murderer; murderer players must concoct lies to hide their identity and avoid detection, while also achieving other objectives in the game.
\paragraph{Rule 3:}Throughout the game, only murderer players are allowed to lie. To conceal their identity, murderers may choose to frame others to absolve themselves of guilt; non-murderer players (civilians) must answer questions from other players and the host honestly and provide as much information as they know about the case to help uncover the truth.
\paragraph{Rule 4:} At the start of the game, each player receives their character script from the host, which contains information about their role and identity.
\paragraph{Rule 5:} Other players cannot see the content of each player's character script, so players must and can only collect information about other players through interaction after the game starts.
\paragraph{Rule 6:} In the voting phase, each player needs to cast their vote for who they think is the murderer in each case. If the player with over 50\% of the votes is the murderer, the civilian players win. Otherwise, the murderer players win.

\subsection{Procedure}

\paragraph{Stage 1: Distribution of Character Scripts}

The host distributes character scripts to each player. These scripts contain the player's name, role (murderer or civilian), and a brief character backstory.

\paragraph{Stage 2: Self-Introduction Session}

Players introduce their characters to the group, laying the groundwork for the game's interactions.

\paragraph{Stage 3: Rounds of Open Questioning}

The game progresses through three rounds of open questioning. Players take turns to ask and answer questions, aiming to gather information about others.

\paragraph{Stage 4: Voting}

In this stage, players vote anonymously to determine their suspicions regarding the identity of the murderer. Each player has one vote.

\paragraph{Stage 5: Outcome Reveal}

The game concludes with the announcement of the voting results, revealing whether the civilian players successfully identified the murderer or not.

\subsection{Example: Solitary Boat Firefly Script}

As an illustrative example, we examine the \textit{Solitary Boat Firefly} murder mystery script, involving six players: [ ``Tian Chou", ``Zhou Lianyi", ``Xi Yan", ``Yu Sunian", Yannan", and ``Zhou Chitong" ], along with four victims: [ ``Zhou Mengdang", ``Bao Liu", ``Cui Shouheng", and ``Wang Xi Rong" ]. We model these characters through a set of agents, denoted as \(\mathcal{A} = \{a_i\}_{i=1}^{N_a}\), where \(N_a=6\) corresponds to the number of players. In parallel with the four victims, we define a set of victims \(\mathcal{V} = \{v_k\}_{k=1}^{N_v}\), where \(N_v=4\), representing the total number of victims in the scenario.

Taking a closer look at ``Tian Chou", depicted as the murderer player \(a_1\), responsible for the demise of two among the four victims, her characterization unfolds as follows:

\begin{itemize}
    \item \textbf{Character Background (\(C_1\))}: "Originating from the Sun lineage, you are endearingly called 'Tian'er'. Your birth year was the twelfth of Guangxu's reign during the Qing Dynasty (1886), marking the beginning of a life filled with extraordinary episodes..."
    
    \item \textbf{Suspicion State (\(s_ijk\))}: The script features four victims, each harbouring suspicions towards the remaining five players. Consequently, \(s_i\) is represented as a $4 \times 5$ matrix, with each row corresponding to a victim and each column reflecting the suspicions they hold against other players. For example, a first row of $[1,0,0,1,0]$ signifies that victim ``Cui Shouheng" suspects both ``Zhou Lianyi" and ``Yannan". So we can get $suspect\_list$ of victim ``Cui Shouheng" is [``Zhou Lianyi" ,``Yannan"] 
    
    \item \textbf{Individual Objectives (\(o_i\))}: The personal objectives for Tian Chou include:
    \begin{enumerate}
        \item Concealing that you killed ``Zhou Mengdang".
        \item Concealing that you killed ``Bao Liu".
        \item Find out the truth about ``Taitai's death".
        \item Conceal your relationship with ``Zhou Chitong".
        \item ...
    \end{enumerate}
\end{itemize}

\subsection{Comparison  Models} \label{appendix:Compare Model}

In this section, we provide a detailed overview of the methodologies compared in our study. Given the game's rules and questioning sequence in our comparisons, we segment the discussion into two phases: the questioning phase and the answering phase.

% Considering the strategic core of the game, a direct confession from the murderer would compromise its competitive nature. Hence, in all the methodologies we explore, we maintain that the murderer's responses follow a predefined template, detailed in \ref{appendix:question reply}. This method preserves the game's integrity and level of challenge.
\begin{enumerate}
    \item \textbf{Werewolf}\citep{werewolf-xu2023}
    
    \textit{Question Generation:} 
    \begin{enumerate}[label=\alph*.]
        \item Selecting questions from a predefined question written by the human specialist, based on the current dialogue and script. The list of expertly devised questions is presented in Table~\ref{tab: predefined question}.
        \item Formulating questions by the selected predefined questions and the ongoing dialogue and script.
    \end{enumerate}
    
    \textit{Answering Questions:}
    \begin{enumerate}[label=\alph*.]
        \item Responding based on the current script and dialog history.
        \item Reflecting on the initial response in light of the dialog history.
        \item Generating the final answer after reflection.
    \end{enumerate}
    
    \item \textbf{Objective-Guided Chain of Thought (O-CoT)}\citep{generative-agent-park2023, narrativeplay-zhao2024}
    
    \textit{Question Generation:} Entails two critical steps:
    \begin{enumerate}[label=\alph*.]
        \item Sequentially reflecting on whether current objectives have been met, with considerations spanning multiple goals such as identifying the murderer, uncovering hidden relationships, or concealing facts. For example, Who is the murderer?
        \item Crafting questions based on these reflections and the current narrative and dialogue.
    \end{enumerate}
    
    \textit{Answering Questions:} 
    \begin{enumerate}[label=\alph*.]
        \item Answers are formulated leveraging the narrative and dialog history.
    \end{enumerate}
    
    \item \textbf{ThinkThrice}\citep{murdergame-wu2024}
    
    \textit{Question Generation:} 
    \begin{enumerate}[label=\alph*.]
        \item Questions are generated based on the script and dialog history.
    \end{enumerate}
    
    \textit{Answering Questions:} 
    \begin{enumerate}[label=\alph*.]
        \item Extracting timelines relevant to the victim.
        \item Evaluating each timeline's relevance to answering the question.
        \item Responding based on the dialog history, character relationships, and the relative script.
        \item Ensuring timelines that aid in answering the question are included in the response. If these are initially missed, the model will later augment and clarify the answer with the required timelines.
    \end{enumerate}

    \item \textbf{The PP (Personal Perspective)}

    The PP assesses agents' performance when limited solely to their scripts, serving as a baseline for initial search efforts. 

    \item \textbf{The OP (Omniscient Perspective)}
    
    The OP evaluates performance under conditions of unrestricted access to all scripts, representing an ideal search endpoint.
    
\end{enumerate}

% Additionally, we assessed the performance of agents that engage passively by directly accessing their scripts (Personal Perspective) or the scripts of all agents (Omniscient Perspective).

% \textit{The PP (Personal Perspective)} assesses agents' performance when limited solely to their scripts, serving as a baseline for initial search efforts. 

% \textit{The OP (Omniscient Perspective)} evaluates performance under conditions of unrestricted access to all scripts, representing an ideal search endpoint.

\subsection{Sensors} \label{appendix:sensor}

This section provides a detailed explanation of the sensors, which are essential for both the Search by Questioning and Action Space Refinement components.

\begin{itemize}
    \item \textbf{Emotion Sensor:} Assesses emotional inclination towards a character. Used in both Search by Questioning and Action Space Refinement. It categorises emotional inclination into ``Positive", ``Neutral", or ``Negative".
    
    \item \textbf{Motivation Sensor:} Evaluates the character's relationship with the victim and the presence of a motive for the crime. It is active in both phases, with choices being ``Yes" or ``No".
    
    \item \textbf{Suspicion Sensor:} Determines if a character is a suspect by analysing their opportunity to commit the crime. It applies to both stages, with responses ``Yes" or ``No".
    
    \item \textbf{Information Value Sensor:} Exclusive to Action Space Refinement, it estimates the probability of obtaining valuable information from further questioning. The choices are ``High", ``Medium", or ``Low".
\end{itemize}

\begin{lstlisting}[mathescape=true]

{
  {
    "(*@\textbf{name}@*)": "emotion",
    "(*@\textbf{for\_Search\_by\_Questioning}@*)": True,
    "(*@\textbf{for\_Action\_Space\_Refinement}@*)": True,
    "(*@\textbf{sensor\_prompt}@*)": "What is your emotional inclination towards the character mentioned above?",
    "(*@\textbf{choices}@*)": ["Positive", "Natural", "Negative"],
  }
  {
    "(*@\textbf{name}@*)": "motivation",
    "(*@\textbf{for\_Search\_by\_Questioning}@*)": True,
    "(*@\textbf{for\_Action\_Space\_Refinement}@*)": True,
    "(*@\textbf{sensor\_prompt}@*)": "What do you think is the relationship between the character mentioned above and the victim? \n  Do you think the character mentioned above has a motive for the crime?",
    "(*@\textbf{choices}@*)": ["Yes", "No"],
  }
  {
    "(*@\textbf{name}@*)": "suspicion",
    "(*@\textbf{for\_Search\_by\_Questioning}@*)": True,
    "(*@\textbf{for\_Action\_Space\_Refinement}@*)": True,
    "(*@\textbf{sensor\_prompt}@*)": "Do you think the character mentioned above is a suspect? \n  This refers to whether the character objectively had the opportunity to commit the crime, such as if someone saw the character at the scene of the crime.",
    "(*@\textbf{choices}@*)": ["Yes", "No"],
  }
  {
   "(*@\textbf{name}@*)": "information value",
    "(*@\textbf{for\_Search\_by\_Questioning}@*)": False,
    "(*@\textbf{for\_Action\_Space\_Refinement}@*)": True,
    "(*@\textbf{sensor\_prompt}@*)": "What do you think is the probability of obtaining valuable information by continuing to question the character mentioned above?",
    "(*@\textbf{choices}@*)": ["High", "Medium", "Low"],
  }
}
\end{lstlisting}

\subsection{Prompt}
\subsubsection{System Prompt}
\paragraph{System Prompt}
designed to introduce the gameplay of the MMG, along with providing essential information about the agents involved. The prompts dynamically adapt to include  \{character\_name\}, representing the agent's character in the game, and \{character\_name\_list\}, listing the characters played by other participants.

For Civilian Players:

\begin{lstlisting}[mathescape=true]
You are playing a game called "Murder Mystery" with other players, which is based on textual interaction. Here are the game rules:

Rule 1: The total number of players participating in the game depends on the script. There may be one or more players who are the murderer(s), while the rest are civilians.
Rule 2: The goal of the game is for civilian players to collaborate and face a meticulously planned murder case together, collecting evidence and reasoning to identify the real murderer among the suspects, all the while ensuring they are not mistaken for the murderer; murderer players must concoct lies to hide their identity and avoid detection, while also achieving other objectives in the game.
Rule 3 Throughout the game, only murderer players are allowed to lie. To conceal their identity, murderers may choose to frame others to absolve themselves of guilt; non-murderer players (civilians) must answer questions from other players and the host honestly and provide as much information as they know about the case to help uncover the truth.
Rule 4: At the start of the game, each player receives their character script from the host, which contains information about their role and identity.
Rule 5: Other players cannot see the content of each player's character script, so players must and can only collect information about other players through interaction after the game starts.
Rule 6: In the voting phase, each player needs to cast their vote for who they think is the murderer in each case. If the player with the most votes is the murderer, the civilian players win. Otherwise, the murderer players win.


Gameplay:
The game has one or more acts. At the beginning of the game, players introduce themselves according to the script, and in each act, you will receive more plot information. In each act, you can ask questions, share your observations, or make deductions to help solve the murder case.
The goal is to identify the true murderer and explain their motive. If you are the true murderer, you must hide your identity and avoid detection.
    
Now, you are playing the role of {character_name}, and the other players are {character_name_list}. 
You are not the murderer. Please collaborate with the other civilian players to achieve your personal objective while finding the true culprit!
\end{lstlisting}

For Killer Players, we replace the last paragraph with:
\begin{lstlisting}[mathescape=true]
  You are the murderer who kills {victims}, and you haven't killed anyone else. Please hide the fact that you committed the murder by fabricating lies and other information, and accomplish your personal objective!
\end{lstlisting}

\subsubsection{Gameplay Prompt}

\paragraph{Self-Introduction Prompt}
designed to facilitate introductions based on the agent's script and objectives. Within this prompt, \{current\_script\} represents the character's script, and \{goal\} represents the objectives of the character within that script.

For Civilian Players:

\begin{lstlisting}[mathescape=true]
Your Script is {current_script}.
Your goal is {goal}.
You are not a murderer, so tell more details to help find the murderer.
If you have something to hide, then be sure not to divulge the relevant information! Don't reveal your goals.
Please introduce yourself.
\end{lstlisting}

For  Killer Players:
\begin{lstlisting}[mathescape=true]
Your Script is {current_script}.
Your goal is {goal}.
If you have something to hide, then be sure not to divulge the relevant information!
Please introduce yourself.
You are a murderer, so You can lie to cover yourself!
\end{lstlisting}

\paragraph{Sensor Prompt}
As outlined in sections \ref{agentname Planning Strategy} and \ref{appendix:sensor}, the Sensor Prompt is crafted to collect a wide array of crucial information. Within this framework, the placeholders \{victim\} and \{character\} are employed to reference the victim's name and the agent being questioned, respectively. Meanwhile, \{current\_script\} and \{dialog\_history\} retrieve the script and dialog logs relevant to both the deceased and the agent under scrutiny, utilising the RAG technique. The constructs \{sensor\_Prompt\} and \{choices\} have been formulated in \ref{appendix:sensor} within the Sensor Prompt segment.

For Civilian Players:

\begin{lstlisting}[mathescape=true]
{victim} was murdered, you are not the murderer, you need to try to find the murderer.
Your Script is about {character} is {current_script}.
The dialog history about {character} is {dialog_history}.
Be warned, if it's a murderer's word it might deceive you.
Based on the information above, {sensor}
Please answer {choices} and explain your reasoning in one or two sentences.
\end{lstlisting}

For  Killer Players:
\begin{lstlisting}[mathescape=true]
{victim} was murdered, you are the murderer, but you need to hide yourself, and pretend you're not the murderer.
Your Script is about {character} is {current_script}.
The dialog history about {character} is {dialog_history}.
Based on the information above, {sensor}
Please answer {choices} and explain your reasoning in one or two sentences.
\end{lstlisting}

\paragraph{Search by Questioning Prompt}
As outlined in sections \ref{agentname Planning Strategy}, the Search by Questioning Prompt is developed based on data acquired from sensors. It includes variables like  \{victim\}, \{character\}, \{current\_script\}, \{dialog\_history\}. Additionally, it integrates a summary, \{summary\}, synthesized from the sensor-collected data. The element \{question\_number\} denotes the total questions permitted, with a detailed discussion on the optimal number of questions presented in the \ref{ablation study} chapter.

For Civilian Players:

\begin{lstlisting}[mathescape=true]
{victim} was murdered, you are not the murderer, you need to try to find the murderer.
Your Script is about {character} is {current_script}.
The dialog history about {character} is {dialog_history}.
{summary}
You can ask {character} {question_number} questions. What would you ask? Please include the victim's name in your question when asking, 
Since the murderer will lie, you can ask questions based on the loopholes and contradictions in what they have previously said.
Please respond in the JSON format without any additional comments. 
For example, 
{
  'Question1': 'Your question', 
  'Question2': 'Your question'
}
\end{lstlisting}

For  Killer Players:
\begin{lstlisting}[mathescape=true]
{victim} was murdered, you are the murderer, But you need to hide yourself, pretend you're not a murderer, and ask questions of other people pretending you suspect the other person is a murderer.
Your Script is about {character} is {current_script}.
The dialog history about {character} is {dialog_history}.
{summary}
You can ask {character} {question_number} questions. What would you ask? Please include the victim's name in your question when asking.
Please respond in the JSON format without any additional comments. 
For example, 
{
  'Question1': 'Your question', 
  'Question2': 'Your question'
}
\end{lstlisting}

\paragraph{Action Space Refinement Prompt}
As outlined in sections \ref{agentname Planning Strategy}, the Action Space Refinement prompt serves as a strategic tool for narrowing down the suspect list, effectively reducing the search domain to augment the efficiency and performance of the algorithm. Within this setup, the term \{victim\} refers to the individual who has been harmed, \{summary\} synthesised from the sensor-collected data, and \{character\_suspect\} identifies the roster of individuals under suspicion. Initially, this roster includes all participating agents, excluding the itself.

\begin{lstlisting}[mathescape=true]
{victim} was murdered.
You think {character_suspect} are suspected of killing {victim}, and your reasons for suspecting them are respectively:
{summary}
Please select several people you think are the most suspicious. You can choose one or more, Please try to reduce the number of suspects.
Please respond in the JSON format without any additional comments. 
For example, 
{
  'suspicion': ["character_name1", "character_name2"]
}
\end{lstlisting}

\paragraph{Question Reply Prompt} \label{appendix:question reply}
The Question Reply Prompt is designed for responding to inquiries, where \{character\} denotes the name of the character asking you a question, and \{question\} is the question itself. \{current\_script\} refers to the script extracted using RAG that pertains to both the deceased and the agent being questioned; \{dialog\_history\} is the dialog log related to the deceased and the interrogated agent, also extracted using RAG.

For Civilian Players:

\begin{lstlisting}[mathescape=true]
{character} ask you a question: {question}
Your Script relative to the question is {current_script}.
The dialog history relative to the question is {dialog_history}.
What you need to pay attention to is {goal}.
Be warned, in the dialog history, if it's a murderer's word it might deceive you.
Please answer the question: "{question}" based on the information above.
You are not the murderer, and you need to work hard to find the murderer. Therefore, provide as much information as possible, such as clues related to the timeline, emotional information, etc.
Please answer the questions from a first-person perspective, rather than saying what someone else said.
\end{lstlisting}

For  Killer Players:
\begin{lstlisting}[mathescape=true]
{character} ask you a question : {question}
Your Script relative to the question is {current_script}.
The dialog history relative to the question is {dialog_history}.
What you need to pay attention to is {goal}.
Be warned, in the dialog history, if it's a murderer's word it might deceive you.
Please answer the questions: "{question}" based on the information above.
You are the murderer. Please hide the fact that you killed {victim}. You can fabricate lies.
Please answer the question from a first-person perspective, rather than saying what someone else said.
\end{lstlisting}

\subsubsection{Evaluation Prompt}

\paragraph{Single-Choice Question Template for the Evaluation Stage Prompt}
This template is utilised during the evaluation stage for answering single-choice questions. It incorporates \{current\_script\}, the script related to the question extracted using RAG, and \{dialog\_history\}, the dialog log relevant to the question, also extracted via RAG. \{question\} is the inquiry presented, and \{choices\} are the available options for that question.
\begin{lstlisting}[mathescape=true]
Please answer the questions based on the information in your script and the content of the dialog
Your Script relative to the question is {current_script}.
The dialog history relative to the question is {dialog_history}.
The question is {question}, the choices is {choices}
Let's think about this problem step by step, please provide your reasoning and your choice (only the option number, e.g., 'a')
You must choose one from the options.
Please respond in the JSON format without any additional comments. 
For example, 
{
    "reason": "Your reason", 
    "answer": "a"
}
\end{lstlisting}

\paragraph{Multiple-Choice Question Template for the Evaluation Stage Prompt}
Similar to the single-choice template, this format is designed for responding to multiple-choice questions during the evaluation stage.
\begin{lstlisting}[mathescape=true]
Please answer the questions based on the information in your script and the content of the dialog
Your Script relative to the question is {current_script}.
The dialog history relative to the question is {dialog_history}.
The question is {question}, the choices is {choices}
That is a multiple-choice question.
Let's think about this problem step by step, please provide your reasoning and your choice (only the option number)
You must make a choice from the options.
Please respond in the JSON format without any additional comments. 
For example, 
{
  "reason": "Your reason", 
  "answer": "a,b"
}
\end{lstlisting}

\paragraph{Single-Choice Question Template for OP Prompt}
This template is specifically designed for Omniscient Perspective (OP), distinguishing it from conventional templates by granting access to the scripts of all players. Unlike standard procedures, it leverages the RAG technique to extract pertinent information from each player's script for comprehensive analysis.
\begin{lstlisting}[mathescape=true]
Please answer the questions based on the information in each character's script:
{current_script}
The question is {question}, the choices is {choices}
Let's think about this problem step by step, please provide your reasoning and your choice (only the option number)
You must choose one from the options.
Please respond in the JSON format without any additional comments.
For example, 
{
  "reason": "Your reason", 
  "answer": "a,b"
}
\end{lstlisting}

\paragraph{Multiple-Choice Question Template for OP Prompt}
Similar to the single-choice version, this template is tailored for answering multiple-choice questions under OP conditions.
\begin{lstlisting}[mathescape=true]
Please answer the questions based on the information in each character's script:
{current_script}
The question is {question}, the choices is {choices}
That is a multiple-choice question.
Let's think about this problem step by step, please provide your reasoning and your choice (only the option number)
You must make a choice from the options.
Please respond in the JSON format without any additional comments. 
For example, 
{
  "reason": "Your reason", 
  "answer": "a,b"
}
\end{lstlisting}

\paragraph{For English Dataset} \label{appendix:English dataset}

Due to budgetary constraints, we only evaluated four scripts from the English dataset, with the performance results reported in Table~\ref{tab:main-results-en}.
For the same scripts, we found that the experiments conducted on the English corpus corroborate the results obtained from the Chinese corpus. Additionally, we observed that the performance of agents based on the English corpus surpassed those based on the Chinese corpus, showing the differential inferencing abilities of LLMs across languages. This discrepancy could be attributed to language biases inherent in the training data utilised for these models.

\begin{table*}[h]
\centering
\resizebox{0.9\linewidth}{!}{
\begin{tabular}{ccccccccc}
\toprule
\multicolumn{1}{c}{\multirow{2}{*}{\textbf{Script}}} & \multirow{2}{*}{\textbf{Evaluation}} & \multicolumn{1}{c}{\multirow{2}{*}{\textbf{\#QA}}} & \multicolumn{1}{c}{\multirow{2}{*}{\textbf{PP}}} & \multicolumn{1}{c}{\multirow{2}{*}{\textbf{OP}}} & \multicolumn{4}{c}{\textbf{Agent's Response After Playing the Game}}    \\ \cmidrule(lr){6-9}
\multicolumn{1}{c}{}                                 &                                      & \multicolumn{1}{c}{}                                      & \multicolumn{1}{c}{}                              & \multicolumn{1}{c}{}                              & \multicolumn{1}{c}{\textbf{Werewolf}} & \multicolumn{1}{c}{\textbf{O-CoT}} & \multicolumn{1}{c}{\textbf{ThinkThrice}} & \multicolumn{1}{c}{\textbf{\agentname \ }} \\
\midrule
\multirow{4}{*}{\shortstack[c]{\emph{Death Wears White}\\ \emph{(9 players, 1 victim)}}}
&  Objective   & $ 10 $ & $.200_{\pm.173}$ & $.900_{\pm.100}$ & $.300_{\pm.100}$ & $.267_{\pm.058}$ & $.300_{\pm.000}$ & $.267_{\pm.058}$ \\
&  Reasoning    & $ 102 $ & $.350_{\pm.044}$ & $.520_{\pm.026}$ & $.356_{\pm.037}$ & $.363_{\pm.049}$ & $.399_{\pm.006}$ & $.441_{\pm.030}$ \\
&  Relations    & $ 72 $ & $.547_{\pm.008}$ & $.445_{\pm.026}$ & $.495_{\pm.016}$ & $.495_{\pm.057}$ & $.398_{\pm.032}$ & $.491_{\pm.021}$ \\
&  Overall      & $ 184 $ & $.367_{\pm.040}$ & $.549_{\pm.012}$ & $.375_{\pm.033}$ & $.375_{\pm.026}$ & $.385_{\pm.010}$ & $.427_{\pm.029}$ \\
\midrule
\multirow{4}{*}{\shortstack[c]{\emph{Ghost Revenge}\\ \emph{(7 players, 3 victims)}}}
&  Objective   & $ 19 $ & $.403_{\pm.061}$ & $.561_{\pm.132}$ & $.439_{\pm.109}$ & $.211_{\pm.106}$ & $.211_{\pm.106}$ & $.526_{\pm.106}$ \\
&  Reasoning    & $ 152 $ & $.456_{\pm.004}$ & $.507_{\pm.007}$ & $.439_{\pm.031}$ & $.539_{\pm.023}$ & $.441_{\pm.017}$ & $.423_{\pm.031}$ \\
&  Relations    & $ 69 $ & $.309_{\pm.009}$ & $.261_{\pm.025}$ & $.328_{\pm.059}$ & $.304_{\pm.015}$ & $.280_{\pm.017}$ & $.353_{\pm.059}$ \\
&  Overall      & $ 240 $ & $.428_{\pm.010}$ & $.485_{\pm.024}$ & $.425_{\pm.002}$ & $.452_{\pm.023}$ & $.380_{\pm.010}$ & $.432_{\pm.013}$ \\
\midrule
\multirow{4}{*}{\shortstack[c]{\emph{Danshui Villa}\\ \emph{(7 players, 2 victims)}}}
&  Objective   & $ 12 $ & $.167_{\pm.083}$ & $.278_{\pm.048}$ & $.472_{\pm.048}$ & $.333_{\pm.000}$ & $.305_{\pm.048}$ & $.389_{\pm.096}$ \\
&  Reasoning    & $ 128 $ & $.325_{\pm.031}$ & $.427_{\pm.009}$ & $.401_{\pm.020}$ & $.373_{\pm.020}$ & $.344_{\pm.014}$ & $.357_{\pm.033}$ \\
&  Relations    & $ 63 $ & $.328_{\pm.056}$ & $.460_{\pm.028}$ & $.391_{\pm.066}$ & $.312_{\pm.106}$ & $.376_{\pm.046}$ & $.407_{\pm.075}$ \\
&  Overall      & $ 203 $ & $.292_{\pm.012}$ & $.412_{\pm.017}$ & $.409_{\pm.009}$ & $.359_{\pm.010}$ & $.343_{\pm.010}$ & $.369_{\pm.033}$ \\
\midrule
\multirow{4}{*}{\shortstack[c]{\emph{Unfinished Love }\\ \emph{(7 players, 2 victims)}}}
&  Objective   & $ 12 $ & $.167_{\pm.000}$ & $.195_{\pm.048}$ & $.389_{\pm.048}$ & $.417_{\pm.000}$ & $.361_{\pm.048}$ & $.528_{\pm.127}$ \\
&  Reasoning    & $ 61 $ & $.536_{\pm.018}$ & $.557_{\pm.028}$ & $.650_{\pm.038}$ & $.612_{\pm.009}$ & $.634_{\pm.038}$ & $.656_{\pm.000}$ \\
&  Relations    & $ 72 $ & $.491_{\pm.016}$ & $.551_{\pm.016}$ & $.509_{\pm.032}$ & $.481_{\pm.021}$ & $.592_{\pm.008}$ & $.500_{\pm.037}$ \\
&  Overall      & $ 145 $ & $.446_{\pm.006}$ & $.479_{\pm.029}$ & $.560_{\pm.011}$ & $.538_{\pm.010}$ & $.566_{\pm.009}$ & $.589_{\pm.018}$ \\

\bottomrule
\end{tabular}}
\caption{Compare the performance of agents with other multi-agent algorithms designed for multiplayer deduction games. PP and OP stand for Personal Perspective and Omniscient Perspective, respectively, representing the performance of agents when they have access to either only their own script or the scripts of all agents, without interacting with other agents.} 
\label{tab:main-results-en}                       
\end{table*}

\begin{table*}[ht!]
\centering
\resizebox{0.8\linewidth}{!}{
\begin{tabular}{cl}
\toprule
\textbf{Index} & \multicolumn{1}{c}{\textbf{Question}} \\ 
\midrule
1 & What was your timeline on the day of the incident? \\
2 & How would you describe your relationship with the victim? \\
3 & When was the last time you saw the victim?  \\
4 & Do you know if the victim had any enemies or conflicts with anyone? \\
5 & What details or anomalies did you notice at the scene of the crime? \\
6 & Did the victim mention anything to you or others that made them worried or fearful recently? \\
7 & Did you notice any unusual people or behaviors on the day of the incident? \\
8 & How much do you know about the victim's secrets or personal life? \\
9 & Were there any items or remains found at the crime scene that could be related to the crime? \\
10 & Do you have any personal opinions or theories about the case? \\ \bottomrule
\end{tabular}
}

\caption{Predefined questions for Werewolf method.}
\label{tab: predefined question}
\end{table*}

\begin{table*}[ht!]
\centering
\resizebox{\linewidth}{!}{
\begin{tabular}{p{0.05\linewidth} p{0.19\linewidth} p{0.19\linewidth} p{0.19\linewidth} p{0.19\linewidth} p{0.19\linewidth}}
\toprule
\textbf{Score} & \textbf{Story Advancement} & \textbf{Question Quality} & \textbf{Response Quality} & \textbf{Role Immersion} & \textbf{Response Speed} \\
\midrule
5  & Actively gathers information and conducts in-depth analyses. Reasoning is rigorous, offering key insights that significantly advance the narrative. & Poses highly relevant, in-depth questions that directly propel the plot and uncover hidden clues. & Provides accurate and comprehensive responses fully aligned with the character’s background and narrative needs. Offers clear, valuable information. & Fully embodies the character. Actions, dialogue, and emotional expressions are authentically aligned with the character’s traits, leaving a strong impression. & Responds promptly with no perceptible delay. The thought process is fluid and maintains a brisk, engaging pace. \\[5pt]

4  & Proactively seeks information and performs reasonable analysis. Reasoning is generally accurate and supports narrative progression. & Most questions are relevant and yield useful information. Occasionally introduces innovative queries. & Generally provides accurate and sufficiently complete answers. Minor omissions occur but do not hinder overall understanding. & Frequently demonstrates character traits. Occasionally shows minor deviations, but emotional expression is largely appropriate. & Responds relatively quickly with brief, occasional delays. The thought process is mostly smooth and well-paced. \\[5pt]

3  & Participates in information gathering but lacks analytical depth. Reasoning may be somewhat biased, offering moderate narrative progression. & Some questions are relevant, but lack depth. Occasional repetition or irrelevant queries occur. & Responses are basically accurate but sometimes incomplete or vague. May require further clarification by others. & Occasionally exhibits character traits, but inconsistently. Emotional expression is average, and immersion is limited. & Moderate response speed with some noticeable pauses. The reasoning process is acceptable but not seamless. \\[5pt]

2  & Shows limited initiative in gathering information, with superficial analysis. Reasoning is frequently flawed, hindering effective plot advancement. & Most questions bear little relevance, often fail to obtain valuable clues, and frequently repeat similar inquiries. & Responses are often inaccurate, incomplete, or misleading. Frequent clarification requests from others are necessary. & Characterization is unclear; actions and dialogue often stray significantly from the intended character profile. Emotional expression is awkward or absent. & Responses are slow with frequent delays. The reasoning process is disjointed, disturbing the overall gameplay flow. \\[5pt]

1  & Does not gather information or attempt analysis. Unable to perform meaningful reasoning, leaving the narrative stagnant. & Poses irrelevant or no questions, providing no support for narrative progression. & Responses are unrelated or outright refusals. Offers no assistance in understanding the narrative. & Demonstrates no character immersion; actions and dialogue contradict character traits. No emotional expression is evident. & Extremely slow responses or prolonged silence. The reasoning process halts, severely impeding the game’s progress. \\
\bottomrule
\end{tabular}
}
\caption{Criteria for each evaluation dimension (Story Advancement, Question Quality, Response Quality, Role Immersion, and Response Speed).}
\label{tab:rating-criteria}
\end{table*}

\section{Agent Interaction Examples} \label{agent-vs-human-examples}

To illustrate the effectiveness of our proposed agent, \agentname, we present examples of dialogue records showcasing interactions between human players and agent players. Below are four versions in which the agent-character \emph{Inspector Howard} interrogates \emph{Farmer Jack} about eyewitness details concerning the murder of \emph{Merchant Green}. These versions correspond to different models: \textbf{Werewolf}, \textbf{ThinkThrice}, \textbf{O-CoT}, and \textbf{\agentname}.

\subsection{Dialogue Versions}

\subsubsection{Werewolf} \begin{quote} \emph{Inspector Howard $\rightarrow$ Farmer Jack}: 

``Did you notice any unusual interactions between Merchant Green and other villagers?''

\emph{Farmer Jack replies}:

``No, nothing in particular.'' \end{quote}

\subsubsection{O-CoT} \begin{quote} \emph{Inspector Howard $\rightarrow$ Farmer Jack}: 

``Jack, that night when you went to Merchant Green's house, did you hear any voices or special sounds?''

\emph{Farmer Jack replies}: 

``I didn't hear any voices, but I did hear the sound of a door being kicked, which was very loud and abrupt.'' \end{quote}

\subsubsection{ThinkThrice} \begin{quote} \emph{Inspector Howard $\rightarrow$ Farmer Jack}: 

``That night, did you notice any unusual situations around Merchant Green's house, like arguments or someone leaving?''

\emph{Farmer Jack replies}:

``I heard some sounds, but couldn't see who it was.'' \end{quote}

\subsubsection{\agentname} \begin{quote} \emph{Inspector Howard $\rightarrow$ Farmer Jack}: 

``Jack, that night you saw someone leaving Merchant Green's house, can you recall what that person was wearing, their actions, or their general direction?''

\emph{Farmer Jack replies}:

``Inspector, that night it was very dark, I could only faintly see that the person was wearing dark clothes, moving very quickly towards the back mountain path. I didn't hear any sounds from him, but his footsteps were very hurried.'' \end{quote}

\subsection{Analysis of Models}

\textbf{Story Progression:} \textbf{Questum} significantly enhances story progression by providing key clues such as the perpetrator's dark clothing, rapid movement, and the direction towards the back mountain path. This enriches the narrative by introducing specific elements that can be further investigated. In contrast, \textbf{Werewolf} offers minimal advancement with a vague response denying any unusual interactions. \textbf{ThinkThrice} slightly improves by mentioning heard sounds but lacks actionable details, while \textbf{O-CoT} introduces the sound of a door being kicked but does not provide additional directions for the investigation.

\textbf{Questioning Ability:} \textbf{Questum} demonstrates superior questioning ability by targeting specific details—clothing, actions, and direction—thereby guiding Farmer Jack to provide more focused and relevant information. \textbf{Werewolf} poses an overly broad question that fails to elicit detailed responses. \textbf{ThinkThrice} narrows the focus slightly but remains too general, and \textbf{O-CoT} asks a more specific question but does not explore as many facets as \textbf{Questum}.

\textbf{Answering Ability:} Responses in \textbf{Questum} are notably detailed, offering observations about the perpetrator’s appearance and behavior, which are crucial for the investigation. This contrasts with \textbf{Werewolf}, where the answer is too brief and lacks specific observations. \textbf{ThinkThrice} provides a partial detail about hearing sounds but fails to elaborate further, while \textbf{O-CoT} mentions the sound of a door being kicked but does not add more context or clues.

\textbf{Role Immersion:} \textbf{Questum} excels in role immersion by portraying Farmer Jack as a tense and observant witness, recalling specific details under pressure. This adds depth to his character and makes the interaction more engaging. \textbf{Werewolf}'s response lacks emotional depth, presenting a mechanical denial. \textbf{ThinkThrice}, while slightly more descriptive, still does not convey significant emotional or psychological engagement. \textbf{O-CoT} includes an abrupt sound but does not enhance the character’s emotional state effectively.

\textbf{Questum} outperforms \textbf{Werewolf}, \textbf{ThinkThrice}, and \textbf{O-CoT} across all evaluated dimensions. Its precise and guided questioning prompts comprehensive and relevant answers, thereby advancing the story effectively. Additionally, the detailed responses enhance character immersion, making the narrative more compelling and believable. The comparison underscores the importance of strategic dialogue design in storytelling, where targeted interactions can significantly enrich the narrative experience.

\subsection{Experiments with Open-Source LLMs} \label{appendix:llama}
\begin{table}[h!]
\centering
\resizebox{\linewidth}{!}{
\begin{tabular}{lllll}
\toprule
Models        & Llama2 70b & Llama2 13b & Llama2 7b & gemma 7b \\ \midrule
Overall Score & 0.312      & 0.281      & 0.267     & 0.273    \\ 
\bottomrule
\end{tabular}}
\caption{Compare the performance of \agentname \  method with different open-source LLMS.} 
\label{tab:main-llama}                       
\end{table}

In addition to experimenting with GPT-3.5-turbo-16k 0613, we also explored Llama2 (70b, 13b, 7b) and Gemma 7b. These models were tested using the scenario ``Solitary Boat Firefly", and the overall results are reported in Table~\ref{tab:main-llama}. The findings indicate that all four models scored significantly lower than GPT-3.5, presumably due to the limitations imposed by a 4k context window. This limitation likely hindered the models' ability to encapsulate sufficient relevant information within such a constrained window. After thorough testing, we observed that despite being evaluated on a Chinese dataset, Llama2 70b primarily resorted to English conversations due to its limited proficiency in Chinese. It responded in English even to Chinese prompts. Other models struggled even more with executing the prompts as required. This limitation greatly hindered their performance in complex gaming situations, such as MMGs. Therefore, we decided to exclusively use GPT-3.5 for future experiments, given its ability to navigate these intricate scenarios.

%\section{Result}\label{appendix:Result}

\begin{table*}[h!]
\centering
\resizebox{0.9 \linewidth}{!}{
\begin{tabular}{ccc|cccccc|cccccc}
\toprule
\multicolumn{1}{c}{\multirow{2}{*}{\textbf{Script}}} 
& \multicolumn{1}{c}{\multirow{2}{*}{\textbf{Evaluation}}} 
& \multicolumn{1}{c}{\multirow{2}{*}{\textbf{\#QA}}} 
& \multicolumn{6}{c}{\textbf{ChatGPT 3.5}} 
& \multicolumn{6}{c}{\textbf{Qwen2.5
32B}} \\
\cmidrule(lr){4-9}\cmidrule(lr){10-15}
\multicolumn{1}{c}{} 
& \multicolumn{1}{c}{} 
& \multicolumn{1}{c}{} 
& \textbf{PP} 
& \textbf{OP} 
& \textbf{Werewolf} 
& \textbf{O-CoT} 
& \textbf{ThinkThrice} 
& \textbf{\agentname} 
& \textbf{PP} 
& \textbf{OP} 
& \textbf{Werewolf} 
& \textbf{O-CoT} 
& \textbf{ThinkThrice} 
& \textbf{\agentname} \\

\midrule
\multirow{5}{*}{\shortstack[c]{\emph{Death Wears White}\\ \emph{(9 players, 1 victim)}}}
&  Win Rate  & $ $-$ $ & $.000_{\pm.000}$ & $.667_{\pm.471}$ & $.000_{\pm.000}$ & $.000_{\pm.000}$ & $.000_{\pm.000}$ & $.000_{\pm.000}$ & $.000_{\pm.000}$ & $1.000_{\pm.000}$ & $.000_{\pm.000}$ & $.000_{\pm.000}$ & $.000_{\pm.000}$ & $.000_{\pm.000}$ \\
&   Objective    & $ $ 10 $ $ & $.067_{\pm.047}$ & $.467_{\pm.094}$ & $.033_{\pm.047}$ & $.067_{\pm.047}$ & $.067_{\pm.047}$ & $.033_{\pm.047}$ & $.167_{\pm.094}$ & $.967_{\pm.047}$ & $.033_{\pm.047}$ & $.067_{\pm.047}$ & $.267_{\pm.094}$ & $.200_{\pm.082}$ \\
&   Reasoning     & $ $ 102 $ $ & $.310_{\pm.026}$ & $.503_{\pm.012}$ & $.258_{\pm.024}$ & $.324_{\pm.014}$ & $.327_{\pm.012}$ & $.356_{\pm.030}$ & $.389_{\pm.028}$ & $.735_{\pm.008}$ & $.458_{\pm.009}$ & $.467_{\pm.018}$ & $.441_{\pm.021}$ & $.539_{\pm.008}$ \\
&   Relations     & $ $ 72 $ $ & $.356_{\pm.040}$ & $.425_{\pm.025}$ & $.421_{\pm.024}$ & $.458_{\pm.041}$ & $.384_{\pm.026}$ & $.435_{\pm.017}$ & $.634_{\pm.017}$ & $.861_{\pm.011}$ & $.699_{\pm.029}$ & $.764_{\pm.030}$ & $.764_{\pm.023}$ & $.741_{\pm.036}$ \\
&   Overall       & $ $ 184 $ $ & $.287_{\pm.017}$ & $.480_{\pm.009}$ & $.260_{\pm.007}$ & $.315_{\pm.006}$ & $.303_{\pm.014}$ & $.328_{\pm.026}$ & $.406_{\pm.027}$ & $.790_{\pm.013}$ & $.447_{\pm.013}$ & $.471_{\pm.016}$ & $.480_{\pm.007}$ & $.533_{\pm.009}$ \\
\midrule
\multirow{5}{*}{\shortstack[c]{\emph{Ghost Revenge}\\ \emph{(7 players, 3 victims)}}}
&  Win Rate  & $ $-$ $ & $.000_{\pm.000}$ & $.333_{\pm.000}$ & $.222_{\pm.157}$ & $.111_{\pm.157}$ & $.000_{\pm.000}$ & $.333_{\pm.000}$ & $.444_{\pm.314}$ & $.889_{\pm.157}$ & $.333_{\pm.000}$ & $.000_{\pm.000}$ & $.333_{\pm.000}$ & $.333_{\pm.000}$ \\
&   Objective    & $ $ 19 $ $ & $.158_{\pm.043}$ & $.333_{\pm.108}$ & $.193_{\pm.066}$ & $.158_{\pm.043}$ & $.193_{\pm.025}$ & $.333_{\pm.066}$ & $.333_{\pm.050}$ & $.825_{\pm.066}$ & $.333_{\pm.066}$ & $.088_{\pm.025}$ & $.316_{\pm.043}$ & $.351_{\pm.066}$ \\
&   Reasoning     & $ $ 152 $ $ & $.300_{\pm.011}$ & $.533_{\pm.025}$ & $.307_{\pm.008}$ & $.322_{\pm.019}$ & $.377_{\pm.022}$ & $.353_{\pm.016}$ & $.417_{\pm.025}$ & $.700_{\pm.011}$ & $.452_{\pm.012}$ & $.461_{\pm.027}$ & $.458_{\pm.014}$ & $.511_{\pm.017}$ \\
&   Relations     & $ $ 69 $ $ & $.222_{\pm.025}$ & $.411_{\pm.084}$ & $.314_{\pm.018}$ & $.295_{\pm.018}$ & $.353_{\pm.025}$ & $.353_{\pm.018}$ & $.662_{\pm.025}$ & $.531_{\pm.048}$ & $.671_{\pm.030}$ & $.599_{\pm.018}$ & $.652_{\pm.012}$ & $.686_{\pm.058}$ \\
&   Overall       & $ $ 240 $ $ & $.266_{\pm.016}$ & $.483_{\pm.016}$ & $.288_{\pm.009}$ & $.290_{\pm.016}$ & $.342_{\pm.015}$ & $.350_{\pm.002}$ & $.433_{\pm.015}$ & $.700_{\pm.012}$ & $.459_{\pm.008}$ & $.413_{\pm.022}$ & $.458_{\pm.008}$ & $.505_{\pm.024}$ \\
\midrule
\multirow{5}{*}{\shortstack[c]{\emph{Danshui Villa}\\ \emph{(7 players, 2 victims)}}}
&  Win Rate  & $ $-$ $ & $.000_{\pm.000}$ & $.167_{\pm.236}$ & $.000_{\pm.000}$ & $.000_{\pm.000}$ & $.000_{\pm.000}$ & $.000_{\pm.000}$ & $.333_{\pm.236}$ & $.000_{\pm.000}$ & $.333_{\pm.236}$ & $.500_{\pm.000}$ & $.667_{\pm.236}$ & $.500_{\pm.000}$ \\
&   Objective    & $ $ 12 $ $ & $.056_{\pm.039}$ & $.222_{\pm.104}$ & $.083_{\pm.000}$ & $.111_{\pm.039}$ & $.194_{\pm.039}$ & $.111_{\pm.079}$ & $.361_{\pm.039}$ & $.083_{\pm.000}$ & $.444_{\pm.079}$ & $.361_{\pm.039}$ & $.528_{\pm.171}$ & $.472_{\pm.039}$ \\
&   Reasoning     & $ $ 128 $ $ & $.247_{\pm.004}$ & $.422_{\pm.013}$ & $.286_{\pm.027}$ & $.286_{\pm.019}$ & $.310_{\pm.004}$ & $.286_{\pm.004}$ & $.380_{\pm.019}$ & $.500_{\pm.019}$ & $.372_{\pm.004}$ & $.424_{\pm.029}$ & $.398_{\pm.023}$ & $.440_{\pm.004}$ \\
&   Relations     & $ $ 63 $ $ & $.254_{\pm.047}$ & $.476_{\pm.022}$ & $.312_{\pm.027}$ & $.365_{\pm.045}$ & $.259_{\pm.015}$ & $.296_{\pm.075}$ & $.598_{\pm.052}$ & $.481_{\pm.049}$ & $.577_{\pm.046}$ & $.614_{\pm.020}$ & $.571_{\pm.013}$ & $.571_{\pm.013}$ \\
&   Overall       & $ $ 203 $ $ & $.222_{\pm.014}$ & $.403_{\pm.023}$ & $.263_{\pm.020}$ & $.274_{\pm.015}$ & $.287_{\pm.008}$ & $.264_{\pm.024}$ & $.409_{\pm.016}$ & $.441_{\pm.016}$ & $.411_{\pm.006}$ & $.443_{\pm.022}$ & $.441_{\pm.005}$ & $.463_{\pm.005}$ \\
\midrule
\multirow{5}{*}{\shortstack[c]{\emph{Unfinished Love }\\ \emph{(7 players, 2 victims)}}}
&  Win Rate  & $ $-$ $ & $.000_{\pm.000}$ & $.167_{\pm.236}$ & $.000_{\pm.000}$ & $.000_{\pm.000}$ & $.000_{\pm.000}$ & $.500_{\pm.000}$ & $.000_{\pm.000}$ & $.500_{\pm.000}$ & $.167_{\pm.236}$ & $.333_{\pm.236}$ & $.167_{\pm.236}$ & $.500_{\pm.000}$ \\
&   Objective    & $ $ 12 $ $ & $.139_{\pm.039}$ & $.167_{\pm.068}$ & $.083_{\pm.118}$ & $.028_{\pm.039}$ & $.000_{\pm.000}$ & $.333_{\pm.068}$ & $.194_{\pm.039}$ & $.528_{\pm.079}$ & $.222_{\pm.079}$ & $.250_{\pm.068}$ & $.194_{\pm.039}$ & $.361_{\pm.039}$ \\
&   Reasoning     & $ $ 61 $ $ & $.475_{\pm.013}$ & $.563_{\pm.020}$ & $.443_{\pm.023}$ & $.426_{\pm.035}$ & $.481_{\pm.039}$ & $.536_{\pm.028}$ & $.536_{\pm.028}$ & $.825_{\pm.008}$ & $.530_{\pm.008}$ & $.557_{\pm.027}$ & $.601_{\pm.015}$ & $.590_{\pm.027}$ \\
&   Relations     & $ $ 72 $ $ & $.421_{\pm.026}$ & $.546_{\pm.017}$ & $.472_{\pm.034}$ & $.519_{\pm.036}$ & $.514_{\pm.020}$ & $.560_{\pm.007}$ & $.745_{\pm.013}$ & $.949_{\pm.017}$ & $.764_{\pm.023}$ & $.745_{\pm.007}$ & $.782_{\pm.013}$ & $.778_{\pm.011}$ \\
&   Overall       & $ $ 145 $ $ & $.391_{\pm.006}$ & $.475_{\pm.027}$ & $.374_{\pm.019}$ & $.366_{\pm.009}$ & $.388_{\pm.026}$ & $.499_{\pm.019}$ & $.517_{\pm.011}$ & $.794_{\pm.016}$ & $.524_{\pm.012}$ & $.540_{\pm.013}$ & $.561_{\pm.007}$ & $.589_{\pm.011}$ \\
\midrule
\multirow{5}{*}{\shortstack[c]{\emph{Cruise Incident}\\ \emph{(5 players, 1 victim)}}}
&  Win Rate  & $ $-$ $ & $.000_{\pm.000}$ & $.333_{\pm.471}$ & $.667_{\pm.471}$ & $1.000_{\pm.000}$ & $.667_{\pm.471}$ & $1.000_{\pm.000}$ & $.000_{\pm.000}$ & $1.000_{\pm.000}$ & $.000_{\pm.000}$ & $.000_{\pm.000}$ & $.000_{\pm.000}$ & $.333_{\pm.471}$ \\
&   Objective    & $ $ 4 $ $ & $.000_{\pm.000}$ & $.250_{\pm.204}$ & $.417_{\pm.118}$ & $.500_{\pm.000}$ & $.583_{\pm.312}$ & $.667_{\pm.236}$ & $.083_{\pm.118}$ & $1.000_{\pm.000}$ & $.000_{\pm.000}$ & $.000_{\pm.000}$ & $.000_{\pm.000}$ & $.250_{\pm.204}$ \\
&   Reasoning     & $ $ 24 $ $ & $.417_{\pm.059}$ & $.472_{\pm.052}$ & $.458_{\pm.068}$ & $.444_{\pm.086}$ & $.458_{\pm.059}$ & $.528_{\pm.052}$ & $.694_{\pm.020}$ & $.819_{\pm.020}$ & $.639_{\pm.020}$ & $.708_{\pm.059}$ & $.667_{\pm.000}$ & $.778_{\pm.071}$ \\
&   Relations     & $ $ 30 $ $ & $.211_{\pm.042}$ & $.411_{\pm.083}$ & $.367_{\pm.082}$ & $.422_{\pm.042}$ & $.411_{\pm.016}$ & $.422_{\pm.016}$ & $.678_{\pm.063}$ & $.800_{\pm.047}$ & $.833_{\pm.047}$ & $.789_{\pm.016}$ & $.700_{\pm.027}$ & $.711_{\pm.016}$ \\
&   Overall       & $ $ 58 $ $ & $.285_{\pm.022}$ & $.415_{\pm.065}$ & $.426_{\pm.031}$ & $.448_{\pm.050}$ & $.468_{\pm.068}$ & $.524_{\pm.015}$ & $.579_{\pm.019}$ & $.847_{\pm.024}$ & $.576_{\pm.002}$ & $.602_{\pm.030}$ & $.555_{\pm.007}$ & $.664_{\pm.006}$ \\
\midrule
\multirow{5}{*}{\shortstack[c]{\emph{Sin}\\ \emph{(4 players, 1 victim)}}}
&  Win Rate  & $ $-$ $ & $.000_{\pm.000}$ & $.333_{\pm.471}$ & $.333_{\pm.471}$ & $.000_{\pm.000}$ & $.000_{\pm.000}$ & $.667_{\pm.471}$ & $.000_{\pm.000}$ & $1.000_{\pm.000}$ & $.000_{\pm.000}$ & $.000_{\pm.000}$ & $.000_{\pm.000}$ & $1.000_{\pm.000}$ \\
&   Objective    & $ $ 3 $ $ & $.000_{\pm.000}$ & $.333_{\pm.272}$ & $.333_{\pm.272}$ & $.000_{\pm.000}$ & $.000_{\pm.000}$ & $.444_{\pm.314}$ & $.000_{\pm.000}$ & $1.000_{\pm.000}$ & $.000_{\pm.000}$ & $.000_{\pm.000}$ & $.000_{\pm.000}$ & $1.000_{\pm.000}$ \\
&   Reasoning     & $ $ 20 $ $ & $.433_{\pm.062}$ & $.567_{\pm.024}$ & $.650_{\pm.108}$ & $.467_{\pm.024}$ & $.533_{\pm.047}$ & $.550_{\pm.041}$ & $.533_{\pm.024}$ & $.933_{\pm.024}$ & $.717_{\pm.047}$ & $.550_{\pm.000}$ & $.633_{\pm.047}$ & $.700_{\pm.041}$ \\
&   Relations     & $ $ 21 $ $ & $.349_{\pm.059}$ & $.587_{\pm.081}$ & $.333_{\pm.067}$ & $.571_{\pm.067}$ & $.413_{\pm.090}$ & $.492_{\pm.022}$ & $.667_{\pm.039}$ & $.937_{\pm.022}$ & $.730_{\pm.059}$ & $.889_{\pm.022}$ & $.698_{\pm.045}$ & $.794_{\pm.022}$ \\
&   Overall       & $ $ 44 $ $ & $.337_{\pm.037}$ & $.531_{\pm.043}$ & $.517_{\pm.087}$ & $.411_{\pm.015}$ & $.411_{\pm.043}$ & $.517_{\pm.064}$ & $.473_{\pm.017}$ & $.946_{\pm.012}$ & $.595_{\pm.015}$ & $.537_{\pm.005}$ & $.539_{\pm.038}$ & $.775_{\pm.024}$ \\
\midrule
\multirow{5}{*}{\shortstack[c]{\emph{Deadly Fountain }\\ \emph{(4 players, 1 victim)}}}
&  Win Rate  & $ $-$ $ & $.000_{\pm.000}$ & $.667_{\pm.471}$ & $.000_{\pm.000}$ & $.000_{\pm.000}$ & $.000_{\pm.000}$ & $.000_{\pm.000}$ & $.000_{\pm.000}$ & $1.000_{\pm.000}$ & $.000_{\pm.000}$ & $.000_{\pm.000}$ & $.000_{\pm.000}$ & $.000_{\pm.000}$ \\
&   Objective    & $ $ 3 $ $ & $.000_{\pm.000}$ & $.556_{\pm.157}$ & $.000_{\pm.000}$ & $.000_{\pm.000}$ & $.000_{\pm.000}$ & $.000_{\pm.000}$ & $.000_{\pm.000}$ & $.889_{\pm.157}$ & $.000_{\pm.000}$ & $.000_{\pm.000}$ & $.000_{\pm.000}$ & $.222_{\pm.157}$ \\
&   Reasoning     & $ $ 21 $ $ & $.317_{\pm.192}$ & $.667_{\pm.103}$ & $.381_{\pm.000}$ & $.444_{\pm.098}$ & $.508_{\pm.022}$ & $.587_{\pm.022}$ & $.587_{\pm.022}$ & $.810_{\pm.000}$ & $.540_{\pm.022}$ & $.556_{\pm.022}$ & $.508_{\pm.045}$ & $.587_{\pm.022}$ \\
&   Relations     & $ $ 12 $ $ & $.250_{\pm.068}$ & $.389_{\pm.039}$ & $.250_{\pm.068}$ & $.194_{\pm.039}$ & $.222_{\pm.039}$ & $.333_{\pm.068}$ & $.722_{\pm.142}$ & $.972_{\pm.039}$ & $.583_{\pm.118}$ & $.667_{\pm.136}$ & $.667_{\pm.068}$ & $.667_{\pm.136}$ \\
&   Overall       & $ $ 36 $ $ & $.247_{\pm.126}$ & $.604_{\pm.085}$ & $.289_{\pm.010}$ & $.323_{\pm.060}$ & $.369_{\pm.013}$ & $.438_{\pm.008}$ & $.497_{\pm.015}$ & $.849_{\pm.027}$ & $.444_{\pm.017}$ & $.468_{\pm.025}$ & $.436_{\pm.031}$ & $.530_{\pm.030}$ \\
\midrule
\multirow{5}{*}{\shortstack[c]{\emph{Unbelievable Incident}\\ \emph{(5 players, 1 victim)}}}
&  Win Rate  & $ $-$ $ & $.000_{\pm.000}$ & $.000_{\pm.000}$ & $.000_{\pm.000}$ & $.000_{\pm.000}$ & $.000_{\pm.000}$ & $.000_{\pm.000}$ & $.000_{\pm.000}$ & $1.000_{\pm.000}$ & $.000_{\pm.000}$ & $.000_{\pm.000}$ & $.000_{\pm.000}$ & $.000_{\pm.000}$ \\
&   Objective    & $ $ 4 $ $ & $.083_{\pm.118}$ & $.083_{\pm.118}$ & $.083_{\pm.118}$ & $.000_{\pm.000}$ & $.000_{\pm.000}$ & $.083_{\pm.118}$ & $.000_{\pm.000}$ & $1.000_{\pm.000}$ & $.000_{\pm.000}$ & $.083_{\pm.118}$ & $.083_{\pm.118}$ & $.000_{\pm.000}$ \\
&   Reasoning     & $ $ 24 $ $ & $.375_{\pm.068}$ & $.528_{\pm.052}$ & $.431_{\pm.052}$ & $.278_{\pm.071}$ & $.194_{\pm.071}$ & $.472_{\pm.020}$ & $.292_{\pm.034}$ & $.694_{\pm.039}$ & $.292_{\pm.000}$ & $.319_{\pm.020}$ & $.278_{\pm.020}$ & $.389_{\pm.020}$ \\
&   Relations     & $ $ 15 $ $ & $.400_{\pm.054}$ & $.822_{\pm.083}$ & $.622_{\pm.083}$ & $.733_{\pm.109}$ & $.289_{\pm.126}$ & $.533_{\pm.054}$ & $.822_{\pm.083}$ & $.911_{\pm.031}$ & $.756_{\pm.063}$ & $.822_{\pm.031}$ & $.733_{\pm.000}$ & $.822_{\pm.031}$ \\
&   Overall       & $ $ 43 $ $ & $.318_{\pm.057}$ & $.481_{\pm.016}$ & $.388_{\pm.032}$ & $.291_{\pm.061}$ & $.168_{\pm.034}$ & $.400_{\pm.019}$ & $.314_{\pm.016}$ & $.793_{\pm.020}$ & $.304_{\pm.010}$ & $.349_{\pm.029}$ & $.309_{\pm.033}$ & $.375_{\pm.017}$ \\
\midrule
\multirow{5}{*}{\shortstack[c]{\emph{Desperate Sunshine}\\ \emph{(4 players, 1 victim)}}}
&  Win Rate  & $ $-$ $ & $.000_{\pm.000}$ & $.667_{\pm.471}$ & $.000_{\pm.000}$ & $.000_{\pm.000}$ & $.667_{\pm.471}$ & $1.000_{\pm.000}$ & $.333_{\pm.471}$ & $.000_{\pm.000}$ & $.333_{\pm.471}$ & $.000_{\pm.000}$ & $.667_{\pm.471}$ & $.000_{\pm.000}$ \\
&   Objective    & $ $ 3 $ $ & $.333_{\pm.000}$ & $.556_{\pm.157}$ & $.333_{\pm.000}$ & $.111_{\pm.157}$ & $.556_{\pm.157}$ & $.778_{\pm.157}$ & $.444_{\pm.157}$ & $.333_{\pm.000}$ & $.333_{\pm.272}$ & $.333_{\pm.000}$ & $.556_{\pm.157}$ & $.333_{\pm.000}$ \\
&   Reasoning     & $ $ 18 $ $ & $.519_{\pm.052}$ & $.778_{\pm.079}$ & $.537_{\pm.026}$ & $.630_{\pm.094}$ & $.759_{\pm.052}$ & $.741_{\pm.069}$ & $.704_{\pm.026}$ & $.833_{\pm.045}$ & $.741_{\pm.052}$ & $.778_{\pm.045}$ & $.741_{\pm.026}$ & $.778_{\pm.000}$ \\
&   Relations     & $ $ 36 $ $ & $.500_{\pm.023}$ & $.611_{\pm.039}$ & $.491_{\pm.094}$ & $.574_{\pm.035}$ & $.491_{\pm.047}$ & $.556_{\pm.068}$ & $.769_{\pm.013}$ & $.861_{\pm.023}$ & $.778_{\pm.023}$ & $.815_{\pm.013}$ & $.787_{\pm.013}$ & $.787_{\pm.035}$ \\
&   Overall       & $ $ 57 $ $ & $.483_{\pm.018}$ & $.681_{\pm.038}$ & $.488_{\pm.034}$ & $.528_{\pm.058}$ & $.627_{\pm.032}$ & $.677_{\pm.041}$ & $.688_{\pm.015}$ & $.766_{\pm.030}$ & $.691_{\pm.032}$ & $.722_{\pm.022}$ & $.729_{\pm.007}$ & $.712_{\pm.013}$ \\
\midrule
\multirow{5}{*}{\shortstack[c]{\emph{Riverside Inn}\\ \emph{(4 players, 1 victim)}}}
&  Win Rate  & $ $-$ $ & $.000_{\pm.000}$ & $.667_{\pm.118}$ & $.083_{\pm.118}$ & $.000_{\pm.000}$ & $.083_{\pm.118}$ & $.250_{\pm.204}$ & $.000_{\pm.000}$ & $.750_{\pm.000}$ & $.083_{\pm.118}$ & $.000_{\pm.000}$ & $.000_{\pm.000}$ & $.083_{\pm.118}$ \\
&   Objective    & $ $ 3 $ $ & $.067_{\pm.024}$ & $.500_{\pm.041}$ & $.117_{\pm.024}$ & $.117_{\pm.062}$ & $.117_{\pm.094}$ & $.383_{\pm.062}$ & $.100_{\pm.000}$ & $.733_{\pm.024}$ & $.167_{\pm.047}$ & $.167_{\pm.024}$ & $.133_{\pm.062}$ & $.250_{\pm.041}$ \\
&   Reasoning     & $ $ 18 $ $ & $.248_{\pm.020}$ & $.569_{\pm.015}$ & $.248_{\pm.013}$ & $.312_{\pm.022}$ & $.281_{\pm.011}$ & $.373_{\pm.017}$ & $.358_{\pm.015}$ & $.832_{\pm.011}$ & $.373_{\pm.016}$ & $.339_{\pm.015}$ & $.394_{\pm.007}$ & $.413_{\pm.020}$ \\
&   Relations     & $ $ 18 $ $ & $.454_{\pm.018}$ & $.507_{\pm.012}$ & $.531_{\pm.014}$ & $.541_{\pm.038}$ & $.483_{\pm.030}$ & $.589_{\pm.071}$ & $.734_{\pm.030}$ & $.768_{\pm.031}$ & $.700_{\pm.025}$ & $.705_{\pm.025}$ & $.647_{\pm.018}$ & $.681_{\pm.059}$ \\
&   Overall       & $ $ 39 $ $ & $.239_{\pm.018}$ & $.544_{\pm.019}$ & $.262_{\pm.008}$ & $.304_{\pm.025}$ & $.276_{\pm.024}$ & $.409_{\pm.009}$ & $.358_{\pm.005}$ & $.800_{\pm.009}$ & $.378_{\pm.006}$ & $.357_{\pm.009}$ & $.375_{\pm.007}$ & $.418_{\pm.005}$ \\
\midrule
\multirow{5}{*}{\shortstack[c]{\emph{Solitary Boat Firefly}\\ \emph{(6 players, 4 victims)}}}
&  Win Rate  & $ $-$ $ & $.222_{\pm.157}$ & $.222_{\pm.157}$ & $.222_{\pm.157}$ & $.000_{\pm.000}$ & $.000_{\pm.000}$ & $.000_{\pm.000}$ & $.222_{\pm.314}$ & $.000_{\pm.000}$ & $.333_{\pm.000}$ & $.111_{\pm.157}$ & $.111_{\pm.157}$ & $.556_{\pm.157}$ \\
&   Objective    & $ $ 20 $ $ & $.167_{\pm.000}$ & $.389_{\pm.071}$ & $.250_{\pm.090}$ & $.181_{\pm.039}$ & $.181_{\pm.039}$ & $.250_{\pm.034}$ & $.333_{\pm.059}$ & $.417_{\pm.000}$ & $.389_{\pm.079}$ & $.236_{\pm.098}$ & $.264_{\pm.109}$ & $.472_{\pm.052}$ \\
&   Reasoning     & $ $ 109 $ $ & $.415_{\pm.011}$ & $.393_{\pm.033}$ & $.409_{\pm.004}$ & $.369_{\pm.044}$ & $.453_{\pm.008}$ & $.539_{\pm.027}$ & $.550_{\pm.021}$ & $.566_{\pm.008}$ & $.553_{\pm.013}$ & $.537_{\pm.027}$ & $.602_{\pm.018}$ & $.618_{\pm.018}$ \\
&   Relations     & $ $ 69 $ $ & $.424_{\pm.042}$ & $.640_{\pm.030}$ & $.473_{\pm.028}$ & $.568_{\pm.048}$ & $.439_{\pm.033}$ & $.542_{\pm.027}$ & $.761_{\pm.009}$ & $.780_{\pm.005}$ & $.758_{\pm.030}$ & $.788_{\pm.019}$ & $.739_{\pm.009}$ & $.780_{\pm.014}$ \\
&   Overall       & $ $ 198 $ $ & $.359_{\pm.013}$ & $.434_{\pm.002}$ & $.383_{\pm.024}$ & $.359_{\pm.027}$ & $.387_{\pm.010}$ & $.472_{\pm.028}$ & $.536_{\pm.021}$ & $.568_{\pm.005}$ & $.550_{\pm.015}$ & $.510_{\pm.011}$ & $.546_{\pm.032}$ & $.612_{\pm.023}$ \\
\midrule
\multirow{5}{*}{\shortstack[c]{\emph{Manna}\\ \emph{(6 players, 3 victims)}}}
&  Win Rate  & $ $-$ $ & $.333_{\pm.471}$ & $1.000_{\pm.000}$ & $.000_{\pm.000}$ & $.000_{\pm.000}$ & $.667_{\pm.471}$ & $.333_{\pm.471}$ & $.000_{\pm.000}$ & $1.000_{\pm.000}$ & $.000_{\pm.000}$ & $.000_{\pm.000}$ & $.000_{\pm.000}$ & $1.000_{\pm.000}$ \\
&   Objective    & $ $ 24 $ $ & $.444_{\pm.157}$ & $.889_{\pm.157}$ & $.111_{\pm.157}$ & $.000_{\pm.000}$ & $.556_{\pm.157}$ & $.444_{\pm.157}$ & $.333_{\pm.000}$ & $1.000_{\pm.000}$ & $.000_{\pm.000}$ & $.333_{\pm.000}$ & $.111_{\pm.157}$ & $1.000_{\pm.000}$ \\
&   Reasoning     & $ $ 123 $ $ & $.519_{\pm.026}$ & $.667_{\pm.045}$ & $.463_{\pm.052}$ & $.426_{\pm.026}$ & $.593_{\pm.026}$ & $.648_{\pm.069}$ & $.704_{\pm.026}$ & $.852_{\pm.026}$ & $.648_{\pm.026}$ & $.759_{\pm.026}$ & $.685_{\pm.026}$ & $.815_{\pm.026}$ \\
&   Relations     & $ $ 88 $ $ & $.370_{\pm.094}$ & $.500_{\pm.079}$ & $.444_{\pm.045}$ & $.407_{\pm.069}$ & $.333_{\pm.045}$ & $.444_{\pm.045}$ & $.907_{\pm.026}$ & $.926_{\pm.026}$ & $.778_{\pm.045}$ & $.741_{\pm.069}$ & $.741_{\pm.069}$ & $.815_{\pm.052}$ \\
&   Overall       & $ $ 235 $ $ & $.470_{\pm.030}$ & $.671_{\pm.029}$ & $.391_{\pm.058}$ & $.340_{\pm.005}$ & $.526_{\pm.055}$ & $.562_{\pm.076}$ & $.679_{\pm.019}$ & $.897_{\pm.009}$ & $.553_{\pm.018}$ & $.673_{\pm.005}$ & $.588_{\pm.026}$ & $.850_{\pm.003}$ \\
\midrule
\multirow{5}{*}{\shortstack[c]{Overall}}
&  Win Rate  & $ $-$ $ & $.016_{\pm.022}$ & $.300_{\pm.041}$ & $.127_{\pm.059}$ & $.063_{\pm.022}$ & $.111_{\pm.045}$ & $.222_{\pm.081}$ & $.143_{\pm.103}$ & $.633_{\pm.024}$ & $.175_{\pm.081}$ & $.095_{\pm.039}$ & $.175_{\pm.059}$ & $.349_{\pm.045}$ \\
&    Objective     & $ $  117  $ $ & $.120_{\pm.007}$ & $.370_{\pm.029}$ & $.160_{\pm.020}$ & $.123_{\pm.008}$ & $.162_{\pm.024}$ & $.288_{\pm.021}$ & $.234_{\pm.028}$ & $.641_{\pm.030}$ & $.242_{\pm.049}$ & $.179_{\pm.030}$ & $.245_{\pm.059}$ & $.373_{\pm.031}$ \\
&    Reasoning      & $ $  800  $ $ & $.336_{\pm.007}$ & $.508_{\pm.009}$ & $.343_{\pm.006}$ & $.349_{\pm.012}$ & $.384_{\pm.002}$ & $.423_{\pm.009}$ & $.454_{\pm.016}$ & $.698_{\pm.009}$ & $.471_{\pm.001}$ & $.480_{\pm.015}$ & $.489_{\pm.003}$ & $.536_{\pm.011}$ \\
&    Relations      & $ $  565  $ $ & $.360_{\pm.005}$ & $.513_{\pm.007}$ & $.425_{\pm.008}$ & $.473_{\pm.010}$ & $.405_{\pm.006}$ & $.471_{\pm.009}$ & $.707_{\pm.007}$ & $.771_{\pm.012}$ & $.714_{\pm.006}$ & $.729_{\pm.009}$ & $.705_{\pm.003}$ & $.725_{\pm.011}$ \\
&    Overall        & $ $  1482  $ $ & $.300_{\pm.006}$ & $.484_{\pm.012}$ & $.324_{\pm.004}$ & $.329_{\pm.008}$ & $.347_{\pm.006}$ & $.407_{\pm.006}$ & $.458_{\pm.016}$ & $.700_{\pm.012}$ & $.472_{\pm.010}$ & $.469_{\pm.016}$ & $.482_{\pm.013}$ & $.540_{\pm.013}$ \\
\bottomrule

\end{tabular}}
\caption{Compare the performance of agents with other multi-agent algorithms designed for multiplayer deduction games. PP and OP stand for Personal Perspective and Omniscient Perspective, respectively, representing the performance of agents when they have access to either only their own script or the scripts of all agents, without interacting with other agents.} 
\label{tab:main-results}                       
\end{table*}
